# Supplementary material for: Towards Rechargeable Zinc-Air Batteries with Aqueous Chloride Electrolytes
Source: arXiv:1902.04400 ancillary file (2019-02-12)
Supplement: Supplementary file 1 [file Supplementary_Information.pdf]

# Supplementary Information: Towards Rechargeable Zinc-Air Batteries with Aqueous Chloride Electrolytes

Simon Clark,[†,‡,¶] Aroa R. Mainar,[§] Elena Iruin,[§] Luis C. Colmenares,[§] J. Alberto Blázquez,[§] Julian R. Tolchard,[¶] Arnulf Latz,[†,‡,‖] and Birger Horstmann[*,†,‡,‖]

†*German Aerospace Center (DLR) Pfaffenwaldring 3840, 70569 Stuttgart, Germany*

‡*Helmholtz Institute Ulm (HIU) Helmholtzstr. 11, 89081 Ulm, Germany*

¶*Sintef Industry, Richard Birkelands vei 2b, 7034 Trondheim, Norway*

§*CIDETEC Energy Storage, P° Miramón, 196, Donostia-San Sebastián 20014, Spain*

‖*Ulm University (UUlm), Institute for Electrochemistry, Albert-Einstein-Allee 47, 89081 Ulm, Germany*

E-mail: birger.horstmann@dlr.de

Phone: +49 (0)711 68628254

## Test Cell Architecture

Photos of the two custom-built zinc-air cells used in the experimental characterization are shown in Figure S1 below. As discussed in the main text, two cell designs were used: ex-situ (C-EI) and operando pH (C-OpH). The C-EI cell contains 1.1 mL of electrolyte and an electrode separation of 0.9 cm. The C-Oph cell contains 4.4 mL of electrolyte with an electrode separation of 2.8 cm.

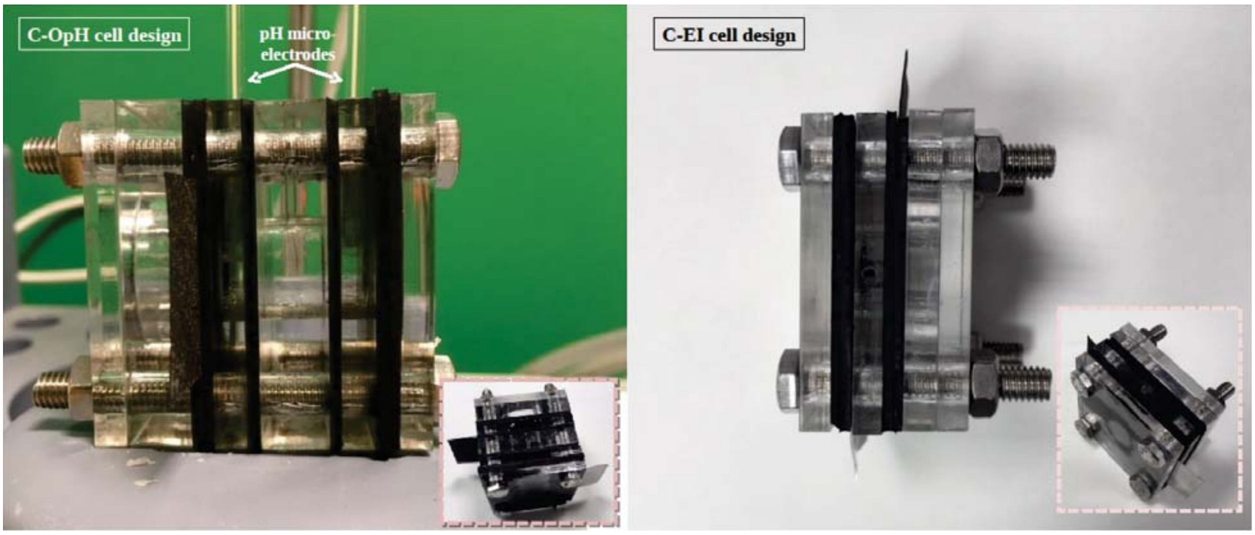


Figure S1: Photos of the C-EI cell (used for full-cell cycling and Zn electrode characterization measurements) and the C-OpH cell (used for operando pH measurements).

# Experimental Results and Discussion

## Full Cell Cycling

Loss of electrolyte contributes to the lifetime limitations during full-cell cycling. It is observed that at the end of the cycling measurement, the cell with electrolyte E8 suffered from significant flooding of the BAE, as shown in Figure S2

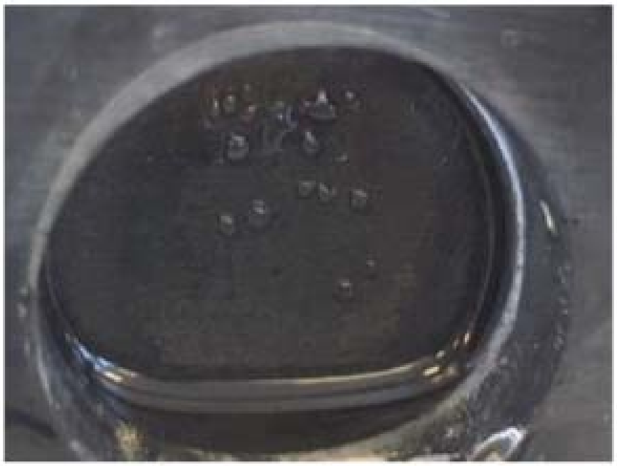

Figure S2: Flooding of the air electrode observed in Cell C-EI with electrolyte E8 at the end of full-cell cycling.

Table S1: EDS elemental characterization for positions labeled "1" and "2" in the SEM images.

| | Discharged | | | | Charged | | | |
|---|---|---|---|---|---|---|---|---|
| | Zn (at%) | Cl (at%) | O (at%) | N (at%) | Zn (at%) | Cl (at%) | O (at%) | N (at%) |
| E4 - Position 1 | 40.9 | 15.7 | 43.5 | 0.0 | 36.4 | 14.0 | 49.7 | 0.0 |
| E4 - Position 2 | 18.8 | 37.4 | 0.0 | 43.8 | 23.1 | 45.4 | 3.3 | 28.2 |
| E6 - Position 1 | 35.7 | 15.4 | 49.0 | 0.0 | 45.3 | 12.2 | 42.6 | 0.0 |
| E6 - Position 2 | 16.1 | 56.5 | 13.4 | 14.0 | 19.4 | 37.2 | 2.9 | 40.5 |
| E7 - Position 1 | 39.8 | 17.5 | 42.7 | 0.0 | 35.0 | 13.7 | 43.5 | 7.8 |
| E7 - Position 2 | 25.6 | 49.8 | 9.2 | 15.4 | 23.5 | 43.5 | 0.0 | 33.0 |
| E8 - Position 1 | 28.4 | 11.4 | 50.6 | 9.7 | 32.1 | 12.8 | 48.5 | 6.7 |
| E8 - Position 2 | 21.1 | 40.8 | 1.1 | 36.9 | 35.6 | 12.9 | 44.9 | 6.7 |

## Zn Electrode Characterization

SEM and EDS measurements of Zn electrodes discharged and charged in electrolytes E4, E7, and E8 are shown below. As noted in the main text, these measurements show two important aspects of zinc precipitate formation in L-ZABs. First, the precipitation during discharge is dominated by mixed zinc hydroxide chloride solids which separate into chlorine-rich and oxygen-rich phases. Second, the precipitated solids do not readily dissolve during charging and in some cases new phases form.

Figure S3 shows the SEM and EDS measurements of Zn electrodes discharged and charged in electrolytes E4, E7, and E8. In electrolyte E4 (a & b), the top view of the discharged electrode shows the separation of chlorine-rich and oxygen-rich phases. The chlorine-rich phase consists of a uniform crystalline domain, while the oxygen-rich phase precipitates as a conglomeration of platelets. The cross section of the charged electrode shows the oxygen-rich layer and chlorine-rich phases forming separate layers.

In electrolyte E7 (Figures S3(b) and (c)), phase layering is also observed in the cross-section of the discharged electrode. In the charged electrode, the top-view measurement shows that the large domains of precipitated solids cover the surface of the electrode.

It is observed that the $ZnCl_2 \cdot 2\,NH_3$ phase tends to form large slab-sided deposits, whereas $ZnCl_2 \cdot 4\,Zn(OH)_2 \cdot H_2O$ forms as plate-type structures. For the precipitates formed in electrolyte E8 and after charging in electrolyte E7, these plate-type structures are apparently

much larger than for the other samples.

The EDS elemental analysis for positions labeled "1" and "2" in the SEM images are presented in Table S1. We note that for electrolytes E6 and E7 after discharge, the atomic ratios for the chlorine-rich phase deviate somewhat from the expected 1:2:2 for Zn:Cl:N, and the phase appears to be more chlorine-rich than the $ZnCl_2 \cdot 2\,NH_3$ identified by the XRD patterns for these samples. This may be due to the formation of additional amorphous or poorly crystalline chlorine-rich phases, or due to only a small quantity of a more chlorine-rich composition being present and thus being below the detection limit of XRD. For precipitates formed in electrolytes E4 and E8 after discharge, and in E4, E6 and E7 after charge, the measured compositions of both chlorine-rich and oxygen-rich phases correspond extremely well to the phases observed by XRD. It is interesting to note that for the samples which exhibit a modified layered phase by XRD, the Zn:Cl:O ratio agrees well with that of $ZnCl_2 \cdot 4\,Zn(OH)_2 \cdot H_2O$, but that these samples are observed to contain a measurable quantity of nitrogen also, which is not the case for the samples in which Simonkolleite was observed.

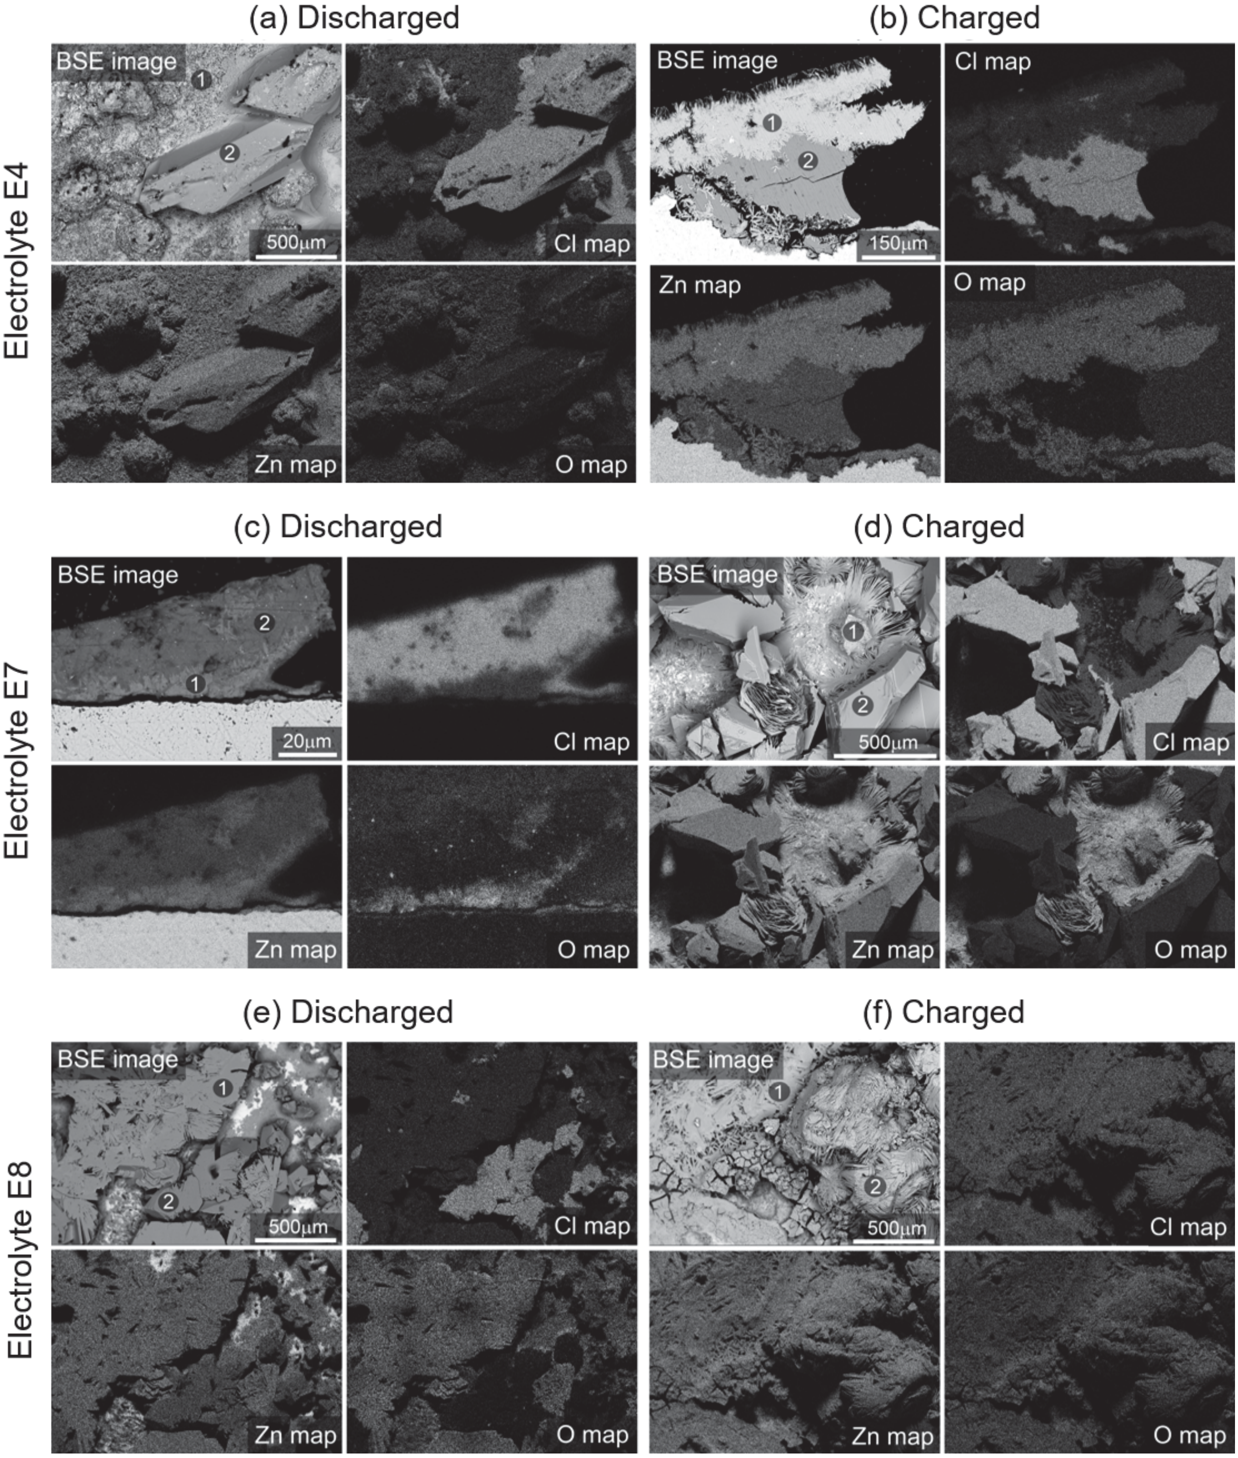


Figure S3: SEM and EDS analysis of Zn electrodes discharged and charged in electrolytes E4 (a & b), E7 (c & d), and E8 (e & f).

# Modeling and Simulation

The modeling approach in this study follows that laid out in existing works,[1–4] with some modifications and improvements described below.

## Thermodynamic Modeling

The models applied to study the speciation, solubility, and equilibrium redox potentials of the L-ZAB system are derived and validated in existing works.[1,5–9] An overview is given below.

According to the law of mass action, for a system at constant temperature and pressure, the value of the reaction quotient is constant. Expressed in terms of a generic reaction, this becomes

$$a\mathrm{A} + b\mathrm{B} \rightleftharpoons c\mathrm{C} + d\mathrm{D}, \qquad \frac{[\mathrm{C}]^c[\mathrm{D}]^d}{[\mathrm{A}]^a[\mathrm{B}]^b} = K, \tag{1}$$

where $K$ is the equilibrium constant of the reaction. Considering the conservation of mass and charge in the electrolyte, the concentration of $n$ solute species described by $r$ homogeneous reactions can be determined from $n - r - 1$ fundamental solute concentrations.[1,2] The homogeneous electrolyte reactions and corresponding equilibrium constants considered in our model are listed in Table S3 in the section *Parameters*.

For a LeClanchè electrolyte ($ZnCl_2$$-$$NH_4Cl$) with the pH adjusted through the addition of $NH_4OH$, there are a total of 28 solutes and 24 homogeneous electrolyte reactions considered in the model. Therefore, 3 fundamental concentrations are needed to describe the system. We choose [$Zn^{2+}$], [$Cl^-$], and [$NH_4^+$]. To calculate the values of these concentrations for a given electrolyte composition, we setup and solve the mass and charge balances for the

system. The zinc and chloride mass conservation equations are:

$$[\mathrm{Zn}]_\mathrm{T} = [\mathrm{Zn}^{2+}] + \sum_{i=1}^{4}[\mathrm{ZnCl_i}^{2-\mathrm{i}}] + [\mathrm{ZnCl_3NH_3}] + [\mathrm{ZnCl(NH_3)_3}] + \sum_{j=1}^{4}[\mathrm{Zn(NH_3)_j}^{2+}] + \sum_{k=1}^{4}[\mathrm{Zn(OH)_k}^{2-\mathrm{k}}] + \sum_{l=1}^{3}[\mathrm{Zn(OH)(NH_3)_l}^{1+}] + \sum_{m=1}^{2}[\mathrm{Zn(OH)_2(NH_3)_m}] + [\mathrm{Zn(OH)_3NH_3}] + [\mathrm{ZnOHCl}], \quad (2)$$

$$[\mathrm{Cl}]_\mathrm{T} = [\mathrm{Cl}^-] + [\mathrm{HCl}] + \sum_{i=1}^{4} i[\mathrm{ZnCl_i}^{2-\mathrm{i}}] + 3[\mathrm{ZnCl_3NH_3}] + [\mathrm{ZnCl(NH_3)_3}] + [\mathrm{ZnOHCl}]. \quad (3)$$

The charge conservation is expressed as:

$$0 = \Big([\mathrm{Cl}]_\mathrm{T} + [\mathrm{OH}]_\mathrm{T}\Big) - \Big(2[\mathrm{Zn}]_\mathrm{T} + [\mathrm{H}]_\mathrm{T}\Big), \quad (4)$$

where,

$$[\mathrm{OH}]_\mathrm{T} = [\mathrm{OH}^-] + \sum_{k=1}^{4} k[\mathrm{Zn(OH)_k}^{2-\mathrm{k}}] + \sum_{l=1}^{3}[\mathrm{Zn(OH)(NH_3)_l}^{1+}] + \sum_{m=1}^{2} 2[\mathrm{Zn(OH)_2(NH_3)_m}] + 3[\mathrm{Zn(OH)_3NH_3}] + [\mathrm{ZnOHCl}], \quad (5)$$

$$[\mathrm{H}]_\mathrm{T} = [\mathrm{H}^+] + [\mathrm{HCl}] + [\mathrm{NH_4}^+]. \quad (6)$$

With the two equations for mass conservation and and equation for charge conservation, the concentrations of $[Zn^{2+}]$, $[Cl^-]$, and $[NH_4^+]$ are calculated.

The solubilities of the various solid precipitates are calculated according to the solubility product constant, $K_{\mathrm{sp}}$. For a generic precipitation reaction:

$$\mathrm{aA + bB + cC \rightleftharpoons A_aB_bC_c(s)}, \qquad K_{\mathrm{sp}} = [A]^a[B]^b[C]^c, \quad (7)$$

where the concentrations are expressed in units of mole·$L^{-1}$. Values for the solubility product

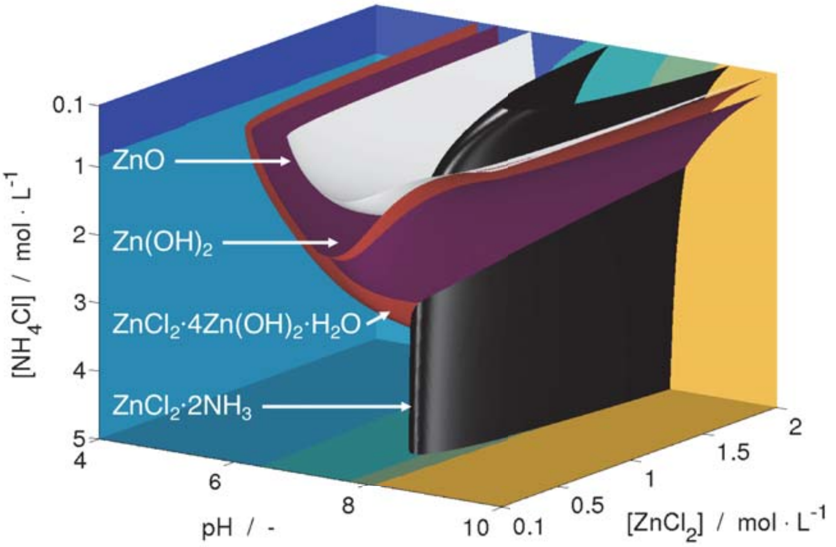


Figure S4: 3D thermodynamic landscape of the $ZnCl_2-NH_4Cl-NH_4OH-H_2O$ electrolyte. The colored regions indicate the dominant zinc complex in the electrolyte, while the colored surfaces show the solubility limits for the various zinc solids considered in the system, as outlined in the main text.

constants are given in Table S4.

Figure S4 shows the 3D speciation and solubility landscape for the LeClanché electrolyte, $ZnCl_2-NH_4Cl-NH_4OH$. The data is plotted as a function of pH, $ZnCl_2$ concentration, and $NH_4Cl$ concentration. The plot shows that in the mildly acidic pH region, zinc is very soluble for all compositions. As the pH increases, a variety of solids including $ZnCl_2 \cdot 4\,Zn(OH)_2 \cdot H_2O$ (red), $ZnCl_2 \cdot 2\,NH_3$ (black), $Zn(OH)_2$ (purple), and ZnO (white) can precipitate. For compositions in which the total amount of chloride present is relatively low, the thermodynamically favored solids are dominated by $ZnCl_2 \cdot 4\,Zn(OH)_2 \cdot H_2O$ and $Zn(OH)_2$. As the total chloride content of the electrolyte increases, $ZnCl_2 \cdot 2\,NH_3$ becomes the dominant solid.

The Nernst equation is used to calculate the concentration-dependent equilibrium redox potential of the various electrochemical reactions in the L-ZAB:

$$E = E^0 - \frac{RT}{zF}\ln Q, \tag{8}$$

where $E^0$ is the standard redox potential and $Q$ is the reaction quotient.

## Quasi-Particle Continuum Modeling

For near-neutral $ZnCl_2-NH_4Cl$ electrolytes, the large quantity of solutes and the orders-of-magnitude concentration shifts that occur make obtaining numerical solutions to the mass and charge continuity equations problematic. Our previous theory-based study of L-ZABs derived a novel method of continuum modeling, based on the use of so-called quasi-particles.[1] Quasi-particles are defined to represent the quantities of mass and charge that are conserved in the homogeneous electrolyte reactions. Solving the continuity equations for these quantities significantly reduces the computational effort required to obtain a solution.

### Definitions

The number of quasi-particles required to describe the system is one less than the difference of the number of solute species and the number of homogeneous reactions ($n_q = n_s - n_r - 1$). In the L-ZAB system, we consider 24 homogeneous reactions and 28 solute species. Therefore, 3 quasi-particles are required. The concentrations of the quasi-particles are defined as the sum of their constituent components, weighted by the stoichiometric coefficient $\tau_{i,q}$ for solute species $i$ in quasi-particle $q$. In this case, we make the following definitions:

$$[\widetilde{\mathrm{Zn}}] = [\mathrm{Zn}^{2+}] + \sum_{i=1}^{4} [\mathrm{ZnCl_i}^{2-\mathrm{i}}] + [\mathrm{ZnCl_3NH_3}] + [\mathrm{ZnCl(NH_3)_3}] + \sum_{j=1}^{4} [\mathrm{Zn(NH_3)_j}^{2+}] + \sum_{k=1}^{4} [\mathrm{Zn(OH)_k}^{2-\mathrm{k}}] + \sum_{l=1}^{3} [\mathrm{Zn(OH)(NH_3)_l}^{1+}] + \sum_{m=1}^{2} [\mathrm{Zn(OH)_2(NH_3)_m}] + [\mathrm{Zn(OH)_3NH_3}] + [\mathrm{ZnOHCl}] \quad (9)$$

$$[\widetilde{\mathrm{NH_3}}] = [\mathrm{NH_3}] + [\mathrm{NH_4}^{+}] + [\mathrm{ZnCl_3NH_3}] + 3[\mathrm{ZnCl(NH_3)_3}] + \sum_{j=1}^{4} j[\mathrm{Zn(NH_3)_j}^{2+}] + \sum_{l=1}^{3} l[\mathrm{Zn(OH)(NH_3)_l}^{1+}] + \sum_{m=1}^{2} m[\mathrm{Zn(OH)_2(NH_3)_m}] + [\mathrm{Zn(OH)_3NH_3}] \quad (10)$$

$$[\widetilde{\mathrm{HOH}}] = \Big([\mathrm{H}^{+}] + [\mathrm{NH_4}^{+}] + [\mathrm{HCl}]\Big) - \Big([\mathrm{OH}^{-}] + \sum_{k=1}^{4} k[\mathrm{Zn(OH)_k}^{2-k}] + \sum_{l=1}^{3} [\mathrm{Zn(OH)(NH_3)_l}^{1+}] + \sum_{m=1}^{2} 2[\mathrm{Zn(OH)_2(NH_3)_m}] + 3[\mathrm{Zn(OH)_3NH_3}] + [\mathrm{ZnOHCl}]\Big) \quad (11)$$

### Source Terms

Because the quasi-particles represent quantities that are conserved in the homogeneous electrolyte reactions, only the heterogeneous (electro)chemical reactions contribute to the quasi-particle source terms.[1]

The kinetics of the electrochemical reactions are described by the Butler-Volmer approximation,

$$k_e = k_0\Big(\exp\Big[\frac{\alpha RT}{nF}\eta\Big] - \exp\Big[-\frac{(1-\alpha)RT}{nF}\eta\Big]\Big), \quad (12)$$

where $k_0$ is the rate constant (linked to the exchange current density), $\alpha$ is the symmetry factor, $\eta$ is the surface overpotential, and the other variables take on their usual meaning.

The kinetics of the precipitation reactions are assumed to be diffusion-limited, and are described by the equation:

$$k_p = \frac{D}{\delta}\frac{[\mathrm{Zn}^{2+}] - [\mathrm{Zn}^{2+}]_{\mathrm{sat}}}{[\mathrm{Zn}^{2+}]_0}. \quad (13)$$

The length of the diffusion layer, $\delta$, is assumed to be 0.0001 m.

The source term for quasi-particle $q$ due to all heterogeneous (electro)chemical reactions

$r$ is given by,

$$\dot{s}_q = \sum_r \sum_i \tau_{i,q} k_r A_r^{\mathrm{sp}}. \tag{14}$$

The specific surface area available for the reaction, $A_r^{\mathrm{sp}}$, is fixed for the air-electrode electrochemical reaction (given by the active area of the catalyst) and is calculated for all other reactions as:

$$A_r^{\mathrm{sp}} = \frac{6}{a_0}(\varepsilon_s(1-\varepsilon_s)), \tag{15}$$

where $\varepsilon_s$ is the appropriate solid volume fraction, and $a_0$ is the diameter of the solid phase pores.

## Transport

There are two types of mass flux that can contribute to transport in metal-air batteries: diffusion-migration flux, $\vec{N}_q^{\mathrm{DM}}$, and convective flux, $\vec{N}_q^{\mathrm{C}}$.[2] The diffusion-migration flux of the quasi-particles is given as,

$$\vec{N}_q^{\mathrm{DM}} = \sum_i \tau_{i,q} \vec{N}_i^{\mathrm{DM}} = \varepsilon_{\mathrm{e}}^{\tilde{\beta}} \sum_i \big(\tau_{i,q} D_i \vec{\nabla} c_i\big) + \sum_i \big(\tau_{i,q} \frac{t_i}{z_i F}\big)\vec{j}. \tag{16}$$

The electrolyte current density, $\vec{j}$, is given by,

$$\vec{j} = \varepsilon_{\mathrm{e}}^{\tilde{\beta}} \big( - \kappa \vec{\nabla} \phi_{\mathrm{e}} - \sum_i \frac{\kappa t_i}{z_i F} \frac{\partial \mu_i}{\partial c_i} \vec{\nabla} c_i \big), \tag{17}$$

where $\varepsilon_{\mathrm{e}}$ is the electrolyte volume fraction, $\tilde{\beta}$ is the Bruggeman coefficient, $t_i$ is the transference number and $z_i$ is the charge number of the solute species, $\kappa$ is the electrolyte conductivity, $\phi_{\mathrm{e}}$ is the electrolyte potential, and $\mu_i$ is the chemical potential of the solute species.

The convective flux is given by,

$$\vec{N}_q^{\mathrm{C}} = \varepsilon_{\mathrm{e}}^{\tilde{\beta}} c_i \vec{v}_{\mathrm{e}}, \tag{18}$$

where $\vec{v}_\mathrm{e}$ is the mass-average velocity of the electrolyte, which is calculated using a Darcy approach:

$$\vec{v}_\mathrm{e} = -\frac{B_\mathrm{e}}{\tilde{\mu}_\mathrm{e}}\vec{\nabla}p_\mathrm{e}. \tag{19}$$

The pressure in the electrolyte is calculated as described in existing works.[1,3,4,10] The equation of state for the electrolyte is,

$$\sum_i \bar{V}_i c_i = 1, \tag{20}$$

where $\bar{V}_i$ is the partial molar volume of the species $i$, and is defined as a material parameter. The link between electrolyte volume fraction and pressure is given through a Leverett-approach. We define the electrolyte saturation of the porous phase as,

$$\tilde{s} = \frac{\varepsilon_\mathrm{e}}{1-\varepsilon_\mathrm{s}}. \tag{21}$$

The capillary pressure is then defined according to the Leverett function,

$$p_\mathrm{c} = p_\mathrm{g} - p_\mathrm{e} = J(\tilde{s}). \tag{22}$$

The dimensionless Leverett function is used to model the pressure saturation characteristics of the porous media. This function takes the form

$$J(\tilde{s}) = A + Be^{C(s-0.5)} - De^{-E(s-0.5)} = \frac{p_\mathrm{c}}{\sigma}\sqrt{\frac{B_0}{\varepsilon_0}}, \tag{23}$$

where $p_c$ is the capillary pressure, $\sigma$ is the surface tension of the electrolyte, $B_0$ is the permeability, and $\varepsilon_0$ is the porosity of the GDE. The coefficients of the Leverett function were determined using a Lattice Boltzmann simulation of a reconstructed GDE structure.[11] We assume that the gas pressure is constant. For more information, please refer to existing works in the literature.[3,4,10]

### Continuity Equations

Considering the quasi-particle definitions, source terms, and transport equations derived above, the equations for mass and charge continuity are

$$\frac{\partial(c_q\varepsilon_{\mathrm{e}})}{\partial t} = -\vec{\nabla}\vec{N}_q^{\mathrm{DM}} - \vec{\nabla}\vec{N}_q^{\mathrm{C}} + \dot{s}_q \tag{24}$$

$$0 = -\vec{\nabla}\vec{j} + \sum_i z_i F \nu_{i,e} k_e A_e^{\mathrm{sp}}, \tag{25}$$

where $\nu_{i,e}$ is the stoichiometric coefficient of solute $i$ in the electrochemical reaction $e$.

## Parameters and Computational Details

This section lists the parameters and computational details utilized in the model. The model is parameterized in conjunction with our existing work.[1] The equilibrium concentrations of the solutes are calculated using the thermodynamic stability constants available in existing works.[5,6,12–14]

Table S2: Parameters of the simulated continuum domains.

| Parameter | C-OpH Cell | C-EI Cell |
|---|---|---|
| Domain Lengths (m) | | |
| $L_{\mathrm{Zn}}$ | $2 \times 10^{-3}$ | $2 \times 10^{-3}$ |
| $L_{\mathrm{Sep}}$ | $28 \times 10^{-3}$ | $9 \times 10^{-3}$ |
| $L_{\mathrm{BAE}}$ | $1 \times 10^{-3}$ | $1 \times 10^{-3}$ |
| Number of Finite Volume Cells (-) | | |
| $N_{\mathrm{Zn}}$ | 20 | 20 |
| $N_{\mathrm{Sep}}$ | 100 | 92 |
| $N_{\mathrm{BAE}}$ | 10 | 10 |
| Initial Solid Volume Fractions (-) | | |
| $\varepsilon_{\mathrm{Zn}}$ | 0.20 | 0.20 |
| $\varepsilon_{\mathrm{Sep}}$ | 0.01 | 0.01 |
| $\varepsilon_{\mathrm{BAE}}$ | 0.30 | 0.30 |
| $\varepsilon_{\mathrm{Precip}}$ | 1e-6 | 1e-6 |

# References


(1) Clark, S.; Latz, A.; Horstmann, B. *ChemSusChem* **2017**, *10*, 4735–4747.

(2) Clark, S.; Latz, A.; Horstmann, B. *Batteries* **2018**, *4*, 5.

(3) Horstmann, B.; Danner, T.; Bessler, W. G. *Energy & Environmental Science* **2013**, *6*, 1299.

(4) Neidhardt, J. P.; Fronczek, D. N.; Jahnke, T.; Danner, T.; Horstmann, B.; Bessler, W. G. *Journal of the Electrochemical Society* **2012**, *159*, A1528–A1542.

(5) Limpo, J.; Luis, A. *Hydrometallurgy* **1993**, *32*, 247–260.

(6) Limpo, J.; Luis, A.; Cristina, M. *Hydrometallurgy* **1995**, *38*, 235–243.

(7) Zhang, Y.; Muhammed, M. *Hydrometallurgy* **2001**, *60*, 215–236.

Table S3: Homogeneous electrolyte reactions and corresponding equilibrium constants.[5,6,12–14]

| Reaction | $\log_{10}\beta$ |
|---|---|
| $H^+ + Cl^- \rightleftharpoons HCl$ | -7.00 |
| $H^+ + NH_3 \rightleftharpoons NH_4^+$ | 9.80 |
| $H^+ + OH^- \rightleftharpoons H_2O$ | 13.96 |
| $Zn^{2+} + Cl^- \rightleftharpoons ZnCl^+$ | 0.72 |
| $Zn^{2+} + 2\,Cl^- \rightleftharpoons ZnCl_2$ | -0.49 |
| $Zn^{2+} + 3\,Cl^- \rightleftharpoons ZnCl_3^-$ | -0.19 |
| $Zn^{2+} + 4\,Cl^- \rightleftharpoons ZnCl_4^{2-}$ | -0.18 |
| $Zn^{2+} + 3\,Cl^- + NH_3 \rightleftharpoons ZnCl_3NH_3^-$ | 3.70 |
| $Zn^{2+} + Cl^- + 3\,NH_3 \rightleftharpoons ZnCl(NH_3)_3^+$ | 7.90 |
| $Zn^{2+} + NH_3 \rightleftharpoons Zn(NH_3)^{2+}$ | 2.38 |
| $Zn^{2+} + 2\,NH_3 \rightleftharpoons Zn(NH_3)_2^{2+}$ | 4.88 |
| $Zn^{2+} + 3\,NH_3 \rightleftharpoons Zn(NH_3)_3^{2+}$ | 7.43 |
| $Zn^{2+} + 4\,NH_3 \rightleftharpoons Zn(NH_3)_4^{2+}$ | 9.65 |
| $Zn^{2+} + OH^- + NH_3 \rightleftharpoons ZnOH(NH_3)^+$ | 9.23 |
| $Zn^{2+} + OH + 2\,NH_3 \rightleftharpoons ZnOH(NH_3)_2^+$ | 10.80 |
| $Zn^{2+} + OH + 3\,NH_3 \rightleftharpoons ZnOH(NH_3)_3^+$ | 12.00 |
| $Zn^{2+} + 2\,OH^- + NH_3 \rightleftharpoons Zn(OH)_2(NH_3)$ | 13.00 |
| $Zn^{2+} + 2\,OH^- + 2\,NH_3 \rightleftharpoons Zn(OH)_2(NH_3)_2$ | 13.60 |
| $Zn^{2+} + 3\,OH^- + NH_3 \rightleftharpoons Zn(OH)_3(NH_3)$ | 14.50 |
| $Zn^{2+} + OH^- + Cl^- \rightleftharpoons Zn(OH)Cl$ | 6.51 |
| $Zn^{2+} + OH^- \rightleftharpoons Zn(OH)^+$ | 6.31 |
| $Zn^{2+} + 2\,OH^- \rightleftharpoons Zn(OH)_2$ | 11.19 |
| $Zn^{2+} + 3\,OH^- \rightleftharpoons Zn(OH)_3^-$ | 14.31 |
| $Zn^{2+} + 4\,OH^- \rightleftharpoons Zn(OH)_4^{2-}$ | 17.70 |

Table S4: Precipitation reactions and solubility product constants for the zinc solids considered in the model.[5,6]

| Reaction | Solubility Product Constant |
|---|---|
| $Zn^{2+} + 2\,OH^- \rightleftharpoons ZnO(s) + H_2O$ | -16.83 |
| $Zn^{2+} + 2\,OH^- \rightleftharpoons Zn(OH)_2$ | -17 |
| $Zn^{2+} + 1.6\,OH^- + 0.4\,Cl^- + H_2O \rightleftharpoons Zn(OH)_{1.6}Cl_{0.4} \cdot H_2O$ | -14.2 |
| $Zn^{2+} + 2\,Cl^- + NH_3 \rightleftharpoons Zn(NH_3)_2Cl_2$ | -6.42 |

Table S5: Transport parameters of aqueous species.[15–22]

| Species | $M_i$ / $g \cdot mol^{-1}$ | $z_i$ / – | $D_i \times 10^9$ / $m^2 \cdot s^{-1}$ | $\lambda_i^0 \times 10^4$ / $S \cdot m^2 \cdot equiv^{-1}$ | $\bar{V}_i \times 10^6$ / $m^3 \cdot mol^{-1}$ |
|---|---|---|---|---|---|
| $H^+$ | 1.0 | +1 | 9.31[15] | 349.8[15] | 0 |
| $OH^-$ | 17.0 | -1 | 5.26[15] | 197.6[15] | -4.18[18] |
| $NH_4{}^+$ | 18 | +1 | 1.95[15] | 73.4[15] | 18.13[16] |
| $NH_3$ | 17 | 0 | 1.94[19] | - | 24.43[16] |
| $Cl^-$ | 35.5 | -1 | 2.03[15] | 76.34[15] | 17.79[16] |
| $Zn^{2+}$ | 65.4 | +2 | 0.71[15] | 53[15] | -24.3[18] |
| $O_2{}^{aq}$ | 32 | 0 | 1.5* | - | 30.38[17] |
| $H_2O$ | 18 | 0 | - | - | 18[20] |
| HCl | - | 0 | - | - | - |
| $ZnCl^+$ | 100.8 | +1 | 1.10[21] | 35* | -1.28[22] |
| $ZnCl_2$ | 136.3 | 0 | 1.10[21] | - | 24.82[22] |
| $ZnCl_3{}^-$ | 171.7 | -1 | 1.10[21] | 35[21] | 53.9[22] |
| $ZnCl_4{}^{2-}$ | 207.2 | -2 | 1.10[21] | 55[21] | 81* |
| $Zn(NH_3)^{2+}$ | 82.4 | +2 | 1.12* | 84.2* | 7.5* |
| $Zn(NH_3)_2{}^{2+}$ | 99.4 | +2 | 1.14* | 85.7* | 39.2* |
| $Zn(NH_3)_3{}^{2+}$ | 116.5 | +2 | 1.09* | 81.5* | 70.9* |
| $Zn(NH_3)_4{}^{2+}$ | 133.5 | +2 | 0.83* | 62.7* | 102.6* |
| $ZnCl_3(NH_3)^-$ | 188.8 | -1 | 1.10* | 41.3* | 86.4* |
| $ZnCl(NH_3)_3{}^+$ | 151.9 | +1 | 1.10* | 41.3* | 97.2* |
| $ZnOH(NH_3)^+$ | 99.4 | +1 | 1.0* | 50* | 10* |
| $ZnOH(NH_3)_2{}^+$ | 116.4 | +1 | 1.0* | 50* | 40* |
| $ZnOH(NH_3)_3{}^+$ | 133.4 | +1 | 1.0* | 50* | 60* |
| $Zn(OH)_2(NH_3)$ | 116.4 | 0 | 1.0* | - | 40* |
| $Zn(OH)_2(NH_3)_2$ | 133.4 | 0 | 1.0* | - | 40* |
| $Zn(OH)_3(NH_3)^-$ | 113.4 | -1 | 1.0* | 30* | 20* |
| Zn(OH)Cl | 6.51 | 0 | 1.0* | - | 1* |
| $Zn(OH)^+$ | 82.4 | +1 | 0.50* | 90.35* | 1* |
| $Zn(OH)_2$ | 99.4 | 0 | 0.50* | - | 20* |
| $Zn(OH)_3{}^-$ | 116.4 | -1 | 0.50* | 90.35* | 40* |
| $Zn(OH)_4{}^{2-}$ | 133.4 | -2 | 0.50* | 90.35* | 60* |

*Estimated

Table S6: Leverett function parameters.[23]

| Coefficient | Value |
|---|---|
| A | 0.1872 |
| B | 0.02523 |
| C | 8.707 |
| D | 0.09515 |
| E | 5.622 |

Table S7: Kinetic parameters for the electrochemical reactions.

| Parameter | Value | Unit |
|---|---|---|
| $k_0^{\mathrm{Zn}}$ | $8 \times 10^{-6}$ | $\mathrm{mol} \cdot \mathrm{m}^{-2} \cdot \mathrm{s}^{-1}$ [24] |
| $\alpha_a^{\mathrm{Zn}}$ | 0.5 | - |
| $\alpha_c^{\mathrm{Zn}}$ | 0.5 | - |
| $A_{\mathrm{sp}}^{\mathrm{Zn}}$ | $f(\varepsilon_{\mathrm{Zn}})$ | $\mathrm{m}^{-2} \cdot \mathrm{m}^{-3}$ |
| $a_0$ | $100 \times 10^{-6}$ | m |
| $k_0^{\mathrm{GDE}}$ | $4 \times 10^{-17}$ | $\mathrm{mol} \cdot \mathrm{m}^{-2} \cdot \mathrm{s}^{-1}$ |
| $\alpha_a^{\mathrm{GDE}}$ | 0.5 | - |
| $\alpha_c^{\mathrm{GDE}}$ | 0.5 | - |
| $A_{\mathrm{sp}}^{\mathrm{GDE}}$ | $4.5 \times 10^{3}$ | $\mathrm{m}^{-2} \cdot \mathrm{m}^{-3}$ |


(8) Vazquez-Arenas, J.; Sosa-Rodriguez, F.; Lazaro, I.; Cruz, R. *Electrochimica Acta* **2012**, *79*, 109–116.

(9) Song, Y.; Hu, J.; Tang, J.; Gu, W.; Fu, Y.; Ji, X. *Journal of The Electrochemical Society* **2017**, *164*, D230–D236.

(10) Stamm, J.; Varzi, A.; Latz, A.; Horstmann, B. *Journal of Power Sources* **2017**, *360*, 136–149.

(11) Danner, T.; Eswara, S.; Schulz, V. P.; Latz, A. *Journal of Power Sources* **2016**, *324*, 646–656.

(12) Smith, R.; Martell, A. *Critical Stability Constants*; Springer: New York, NY, 1976; Vol. 4.

(13) Clever, H. L.; Derrick, M. E.; Johnson, S. a. *Journal of Physical and Chemical Reference Data* **1992**, *21*, 941–1004.

(14) Reichle, R. A.; McCurdy, K. G.; Hepler, L. G. *Canadian Journal of Chemistry* **1975**, *53*, 3841–3845.

(15) Newman, J.; Thmoas-Alyea, K. E. *Electrochemical Systems*, 3rd ed.; John Wiley & Sons: Hoboken, New Jersey, 2004.

(16) Shock, E. L.; Helgeson, H. C. *Geochimica et Cosmochimica Acta* **1988**, *88*, 803–826.

(17) Shock, E. L.; Helgeson, H. C.; Sverjensky, D. a. *Geochimica et Cosmochimica Acta* **1989**, *53*, 2157–2183.

(18) Shock, E.; Sassani, D.; Willis, M.; Sverjensky, D. *Geochimica et Cosmochimica Acta* **1997**, *61*, 907–950.

(19) Frank, M. J. W.; Kuipers, J. a. M.; Swaaij, W. P. M. V. *Journal of Chemical & Engineering Data* **1996**, *41*, 297–302.

(20) Atkins, P.; De Paula, J. *The Elements of Physical Chemistry*, 8th ed.; W.H. Freeman and Company: New York, 2006; pp 791–820.

(21) Rard, J. A.; Miller, D. G. *Journal of Solution Chemistry* **1990**, *19*, 129 – 148.

(22) Sverjensky, D.; Shock, E.; Helgeson, H. *Geochimica et Cosmochimica Acta* **1997**, *61*, 1359–1412.

(23) Danner, T.; Horstmann, B.; Wittmaier, D.; Wagner, N.; Bessler, W. G. *Journal of Power Sources* **2014**, *264*, 320–332.

(24) Huajun, Z.; Zhenghai, G.; Jinhuan, Z. *Hydrometallurgy* **2007**, *89*, 369–373.
